# Supplementary material for: Partially Observable Markov Decision Process Modelling for Assessing Hierarchies
Source: arXiv:1908.07031 source file (2020-12-08)
Supplement: Supplementary file 1 [file supplement.tex]

\documentclass{article}
\usepackage[a4paper, total={6in, 8in}]{geometry}
% The following packages will be automatically loaded:
% amsmath, amssymb, natbib, graphicx, url, algorithm2e
\usepackage[hidelinks]{hyperref}

\usepackage{longtable}% for long tables

\usepackage{graphicx}
\usepackage{booktabs}
\usepackage{subfig}
\usepackage{wrapfig}

% The siunitx package is used by this sample document
% to align numbers in a column by their decimal point.
% Remove the next line if you don't require it.
\usepackage[load-configurations=version-1]{siunitx} % newer version
\usepackage{natbib}

\usepackage{wrapfig}

\usepackage{amsmath}
\usepackage{amssymb}
\usepackage{amsthm}
\usepackage{mathtools}
\usepackage{dsfont}
\usepackage[capitalise]{cleveref}
\usepackage{tikz}
\usepackage{multirow,multicol}
\usepackage{bm}
\usepackage{forest}
\usepackage{tikz}
\usepackage{array}
\usepackage[most]{tcolorbox}
\usepackage{appendix}

\usepackage{algorithm}
\usepackage{algorithmic}

\usetikzlibrary{trees,bayesnet,arrows,automata,positioning}

\usepackage{thmtools}

\tcolorboxenvironment{lemma}{enhanced jigsaw,colback=gray!20,drop shadow}

\tcolorboxenvironment{proposition}{enhanced jigsaw,colback=gray!20,drop shadow}

\tcolorboxenvironment{remark}{enhanced jigsaw,colback=gray!20,drop shadow}

\tcolorboxenvironment{definition}{enhanced jigsaw,colback=white,drop shadow}

\usepackage[affil-sl,auth-sc]{authblk}

\title{POMDP Modelling for Assessing Hierarchies: Supplemental Document}

\author[1]{Weipeng Huang\thanks{weipeng.huang@insight-centre.org}}
\author[2]{Guangyuan Piao\thanks{guangyuan.piao@insight-centre.org}}
\author[1]{Raul Moreno\thanks{raul.moreno.salinas@gmail.com}}
\author[1]{Neil Hurley\thanks{neil.hurley@insight-centre.org}}
\affil[1]{Insight Centre for Data Analytics, School of Computer Science, University College Dublin, Dublin, Ireland}
\affil[2]{Insight Centre for Data Analytics, Data Science Institute, IDA Business Park, Galway, Ireland}

\begin{document}

\maketitle
\input{appendix}

\bibliography{evalmodel}

\end{document}
